# Supplementary material for: DreamHead: Learning Spatial-Temporal Correspondence via Hierarchical Diffusion for Audio-driven Talking Head Synthesis
Source: arXiv:2409.10281 source file (2024-09-16)
Supplement: Supplementary file 1 [file X_suppl.tex]

\clearpage
\setcounter{page}{1}
\maketitlesupplementary

\section{Rationale}

\begin{table}[h]
\caption{Comparison with state-of-the-art methods. }
  \centering
  \resizebox{1\linewidth}{!}{
        \begin{tabular}{lccccc}
        \toprule
     
        Method & NIQE $\downarrow$ & LMD-$v$ $\downarrow$ & LMD $\downarrow$ & Sync $\uparrow$ & MA $\uparrow$ \\
        \midrule
        N = 3 & & & & & \\
        N = 6 & & & & & \\
        N = 9 & & & & & \\
        N = 15 & & & & & \\
        N = 18 & & & & & \\
        \midrule
        DreamHead N=12 (Ours)&\textbf{6.51}&\textbf{1.65}&\textbf{1.35}&\textbf{4.90}&\textbf{0.63} \\
        \bottomrule
        \end{tabular}
}
\label{tab:abla-tb-num}

\end{table}

\begin{table}[ht]
\caption{Comparison with state-of-the-art methods. }
  \centering
  \resizebox{1\linewidth}{!}{
        \begin{tabular}{lccccc}
        \toprule
     
        Method & NIQE $\downarrow$ & LMD-$v$ $\downarrow$ & LMD $\downarrow$ & Sync $\uparrow$ & MA $\uparrow$ \\
        \midrule
        Interval = 10 & 6.58& 1.68&1.35&4.57&0.62 \\
        Interval = 15 & 6.55&1.65&1.35&4.78&0.63\\
        Interval = 25 & 6.54&1.66&1.37&4.58&0.62 \\
        Interval = 30 &6.54&1.65&1.35&4.75&0.63\\
        Interval = 40 &6.55&1.65&1.36&4.73&0.62\\
        Random &6.55&1.70&1.37&4.63&0.62\\
        
        \midrule
        Ground Truth (reference) &6.38&0.00&0.00&6.07&1.00\\
        Interval=20 (Ours) &\textbf{6.51}&\textbf{1.65}&\textbf{1.35}&\textbf{4.90}&\textbf{0.63}\\
        \bottomrule
        \end{tabular}
}
\label{tab:abla-interval}
\end{table}

\subsection{Implementation Details}
In this work, we utilize the Mediapiple~\footnote{https://google.github.io/mediapipe/} to detect $478$ 3D facial landmarks for all videos. To project the detected 3D landmarks to the canonical space through a rigid transformation in Section~\ref{sec:a2l}, we estimate the head pose $H$ using 3DFFA~\cite{guo2020towards}. We resize the input image in landmark-to-image diffusion to $256\times 256$, and the downsampling factor $f$ of the encoding is set as $4$. The length of the denoising step T is set as 1000 for both the audio-to-landmark and landmark-to-image diffusion. In the first hierarchy of audio-to-landmark diffusion, the number of the temporal block is 12. We set the interval $\tau$ between the reference image and the target image as 20. In the audio-to-landmark diffusion, we set the l=300 and l=20 for HDTF and MEAD datasets, respectively, because videos in the HDTF dataset are longer than those in MEAD. We set the frame interval $\tau$ in the landmark-to-image diffusion to $20$ so that it would not learn a shortcut with too close frames.
